# Supplementary material for: ML-Bench: Evaluating Large Language Models and Agents for Machine Learning Tasks on Repository-Level Code
Source: arXiv:2311.09835 source file (2024-08-21)
Supplement: Supplementary file 1 [file appendix.tex]

% This must be in the first 5 lines to tell arXiv to use pdfLaTeX, which is strongly recommended.
%\pdfoutput=1
% In particular, the hyperref package requires pdfLaTeX to break URLs across lines.

\documentclass{article}

% Remove the "review" option to generate the final version.

\usepackage{neurips_2023}
% Standard package includes
\usepackage{times}
\usepackage{latexsym}
% \usepackage[table]{xcolor} 
% Optional math commands from https://github.com/goodfeli/dlbook_notation.
\usepackage{microtype}
\usepackage{amssymb}
\usepackage{mathtools}
\usepackage{nicematrix}
\usepackage{colortbl}
\usepackage{hyperref}
\usepackage{url}
\usepackage{amsfonts}
\usepackage{verbatim}
\usepackage{caption}
\usepackage{longtable}
\usepackage{supertabular}
\usepackage{float}
\usepackage{tabularx}
%%%%%%%%%% custom %%%%%%%%%%
\usepackage{amsmath}
%%%%% for table %%%%%%
\usepackage{graphicx}
\usepackage{xcolor}
\usepackage{multirow}
\usepackage{makecell}
\usepackage{arydshln}
\usepackage{booktabs}
%%%%%%%%%%%%%%%%%%%% 
\usepackage{xspace}
\usepackage{wrapfig}
\usepackage[commandnameprefix=ifneeded]{changes}
\usepackage{enumitem}
\usepackage{xcolor}
\usepackage{xspace}
\usepackage{textcomp}
\usepackage{makecell}
\usepackage{multicol}
\usepackage{lscape} 
\usepackage{siunitx}
\usepackage{algorithm}
\usepackage{algpseudocode}
\setlength{\columnsep}{2em}
\setlength{\parindent}{0em}
\setlength{\parskip}{0.7em}
\usepackage{stfloats}
\usepackage{amssymb}% http://ctan.org/pkg/amssymb
\usepackage{pifont}% http://ctan.org/pkg/pifont
\usepackage{scrextend}
\usepackage{threeparttable}
\usepackage{colortbl}
\usepackage{listings}
\lstset{
basicstyle=\ttfamily\footnotesize,
breaklines=true,
}

\usepackage{subfiles}
\usepackage{array}
\usepackage{latexsym}
\usepackage[T1]{fontenc}
\usepackage[utf8]{inputenc}
\usepackage{microtype}
\usepackage{xurl} % URL typesetting with line breaks
\usepackage{nicefrac}       % compact symbols for 1/2, etc.
\usepackage{changepage}
\usepackage{xargs}
\usepackage{wrapfig,lipsum,booktabs}
\usepackage{longtable}
\usepackage{subcaption}
\usepackage{pgfplots}
\usetikzlibrary{pgfplots.groupplots}
\pgfplotsset{compat=1.3}
\usepackage{tikz}
\usetikzlibrary{patterns}
\usepackage{placeins} % For appendix to make sure floats are all in their respective sections (FloatBarrier)

% For proper rendering and hyphenation of words containing Latin characters (including in bib files)
\usepackage[T1]{fontenc}
% For Vietnamese characters
% \usepackage[T5]{fontenc}
% See https://www.latex-project.org/help/documentation/encguide.pdf for other character sets

% This assumes your files are encoded as UTF8
\usepackage[utf8]{inputenc}

% This is not strictly necessary and may be commented out,
% but it will improve the layout of the manuscript,
% and will typically save some space.
\usepackage{microtype}

% This is also not strictly necessary and may be commented out.
% However, it will improve the aesthetics of text in
% the typewriter font.
\usepackage{inconsolata}
% If the title and author information does not fit in the area allocated, uncomment the following
%
%\setlength\titlebox{<dim>}
%
% and set <dim> to something 5cm or larger.

%\usepackage[table,xcdraw]{xcolor}

%Large Language Models Leverage Open-source Libraries for Machine Learning Tasks}
% \newcommand{\papertitle}[0]{\vspace{-2mm}}

\makeatletter
\AtBeginDocument{%
  \renewcommand{\sectionautorefname}{\S\@gobble}

  \renewcommand{\subsectionautorefname}{\S\@gobble}
}
\makeatother

\definecolor{ao(english)}{rgb}{0.0, 0.5, 0.0}

\usepackage{listings}
\usepackage{xcolor}
\lstset{
    columns=fixed,       
    numbers=left,                                        % 在左侧显示行号
    frame=none,                                          % 不显示背景边框
    backgroundcolor=\color[RGB]{245,245,244},            % 设定背景颜色
    keywordstyle=\color[RGB]{40,40,255},                 % 设定关键字颜色
    numberstyle=\footnotesize\color{darkgray},           % 设定行号格式
    commentstyle=\it\color[RGB]{0,96,96},                % 设置代码注释的格式
    stringstyle=\rmfamily\slshape\color[RGB]{128,0,0},   % 设置字符串格式
    showstringspaces=false,                              % 不显示字符串中的空格
    language=c++,                                        % 设置语言
}
% \title{\raggedright \papertitle}

\begin{document}
% \maketitle
\thispagestyle{plain}

\begin{comment}
\section{\textcolor{red}{Apologies for Incorrect Version of Submission}}

We would like to express our sincerest apologies for the incorrect version of our submitted paper.
Unfortunately, we mistakenly submitted a previous version of the paper that did not contain the updated and finalized version. This oversight was unintentional, and we deeply regret any confusion this may have caused.
Specifically, in the draft submitted, there were two grammatical errors: incomplete sentences found in both the caption of Figure 4 and on line 279, and an incorrect version of the Conclusion section was included.
For correction, we have attached the finalized version of the Conclusion to this correspondence and will make it a point to address all aforementioned issues in the revised version of the paper, which will be submitted during the paper rebuttal stage.
% We hope that this updated version provides the clarity and completeness that was intended in our original submission.
Once again, please accept our deepest apologies for this misstep.

\textbf{Final Version of Conclusion Section}:
Our study evaluates the performance of Large Language Models (LLMs) like GPT-4 in repository-scale code understanding and autonomous code interaction.
Our evaluation includes two setups: \textsc{ML-LLM-Bench} for text-to-code conversion and \textsc{ML-Agent-Bench} for end-to-end task execution. Results show GPT-4 achieving a Pass@5 rate over 50\% in \textsc{ML-LLM-Bench} and a 76.47\% success rate in \textsc{ML-Agent-Bench}, highlighting areas for improvement in handling hallucinations and bash script generation.

% \begin{tikzpicture}[remember picture,overlay,shift={(current page.north west)}]
% \node[anchor=north west,xshift=1.2cm,yshift=-1.25cm]{\scalebox{0.5}[0.5]{\includegraphics[width=5.5cm]{figures/owl-2.png}}};
% \end{tikzpicture}

\vspace{-7mm}

\end{comment}

\input{9-appendix}
\input{11-datasheet}

\clearpage
\bibliography{main}
% \bibliographystyle{acl_natbib}
% \bibliography{main}
% \bibliographystyle{ieeenat_fullname}
\bibliographystyle{plain}
\clearpage

% \nocite{*}

% \listoffigures
% \listoftables

\end{document}
